# Supplementary material for: HARPS: An Online POMDP Framework for Human-Assisted Robotic Planning and Sensing
Source: arXiv:2110.10324 source file (2023-03-28)
Supplement: Supplementary file 1 [file appendix_pseud.tex]

\subsection{Parameterized Sketch Generation}
%Discussion of Need for Auto-labeling
A distinct drawback of human-robot interaction research is the time associated with collecting human subject test data. For this work in particular, the tightly integrated planning and sensing at the core of information gathering problems further complicates the collection of human data, as the POMDP must be run in real-time while simultaneously receiving real-time input from a human. Also, while observations from a given softmax model can be drawn probabilistically to simulate a human response, the motivating problem requires the real-time generation of new softmax models from sketches. Thus gathering large sample sizes becomes extremely time intensive. However, such sample sizes are highly desirable for the purpose of investigating the value of online POMDPs in human-robot teams. 

This section describes the Parameterized Sketching Emuluator Utilizing vertex Downsampling (PSEUD), Developed for the purpose of investigating the response and efficacy online human-interacting POMDPs. PSEUD allows the generation of convex sketched polygons according to a learnable set of parameters, effectively drawing a sketch from a distribution of identically parameterized sketches. In this way, the effect of a human's sketch input on the POMDP can be quantified for a broad variety of possible sketching styles and idiosyncrasies, even those likely to represent rare edge cases in the actual human population.

%Formal definitions and math
A 2D PSEUD sketch is parameterized as the 5-tuple $\{\mathcal{X}, r, \sigma, \lambda, \psi\}$. The centroid $\mathcal{X} = \{x,y\}$ 
%\nisarcomm{in frame of map for $\mathcal{S}$? Also, what coord frame are sketch inputs defined in? are these (w.l.o.g.) assumed to be transformed into the same coords as for $\mathcal{S}$ in the POMDP?} 
and characteristic size $r$ are left as features dependent on a given landmark around which the sketch is being made. Specifically, in this work, both $\mathcal{X}$ and $r$ are defined in the 2D plane corresponding to the target state $s_{t}$, while more generally they are defined whichever state space plane the sketch is being drawn on. The chosen landmark might be a choice from a pre-selected set, or generated autonomously using computer vision object recognition approaches. In either case, $r$ serves as the Gaussian mean distance away from the centroid, with some standard deviation $\sigma$, such that for a given vertex $v$ in a hypothetical sketch object $h$ to be simulated the distance of the vertex from the centroid is drawn from the distribution:
\begin{align}
    |\vec{\mathcal{X}v}| \sim \mathcal{N}(r,\sigma)
\end{align}
Where $|\vec{\mathcal{X}v}|$ denotes the magnitude of the vector from the centroid to $\mathcal{X}$ to the vertex $v$. 
%\nisarcomm{what does $|\vec{\mathcal{X}v}|$ mean?}
The number of vertices $N_{v}$ is distributed according to a shifted Poisson Distribution, with mean $\lambda$. The distribution is shifted uniformly upward by three, with support on $\mathcal{R} \in [3,\infty]$, ensuring that sketches are at a minimum triangles. 
\begin{align}
    N_{v} \sim 3 + Pois(\lambda)
\end{align}

For a given $N_{v}$, the requirement that the angles of a convex polygon sum to $2\pi$ radians reveals a nominal angular distance between each point of $\hat{\Delta \theta} = \frac{2\pi}{N_{v}}$ radians. To capture the irregularity of a sketched polygon, the angular noise parameter $\psi$ is used, such that $\hat{\Delta \theta}$ and $\psi$ specify a Gaussian distribution on angular distance. For a vertex $v$, the angular distance to the next vertex is drawn as 
\begin{align}
    \Delta \theta \sim \mathcal{N}(\hat{\Delta \theta}, \psi)
\end{align}
The process for drawing vertices from the distribution specified by the 5-tuple $\{\mathcal{X}, r, \sigma, \lambda, \psi\}$ is summarized in Algorithm \ref{alg:PSEUD}.

\begin{algorithm}[h!]
\caption{Parameterized Sketching Emulator Utilizing vertex Downsampling}
\begin{algorithmic}[1] \label{alg:PSEUD}
\STATE \textbf{Function:} $PSEUD$
\STATE \textbf{Input:} Centroid $\mathcal{X}$, Radius $r$, Sd $\sigma$, Poisson Mean $\lambda$, Angular Noise $\phi$

\STATE Vertex Set $\{V\} = \emptyset$
\STATE Magnitude List $\textit{mags} = []$
\STATE Angle List $\textit{angles} = []$
%Draw number of vertices 
\STATE $N_{v} \sim 3 + Pois(\lambda)$
%Draw vector mags
%Draw each angular distance

\FOR{$i \in N_{v}$}
    \STATE $\textit{mags}_{i} \sim \mathcal{N}(r,\sigma)$
    \STATE $\textit{angles}_{i} \sim \mathcal{N}(\hat{\Delta \theta}, \psi)$
\ENDFOR

%Normalize angles to 2pi
\STATE angles = Normalize($\textit{angles}$,2$\pi$)

\STATE $\theta = \textit{angles}_{0}$ \#Starting angle
%Assign Vertices
\FOR{$i \in N_{v}$}

    \STATE $V_{i} = \mathcal{X} + [\textit{mags}_{i}cos(\theta),\textit{mags}_{i}sin(\theta)]$
    \STATE $\Delta \theta = \textit{angles}_{i}$
    \STATE $\theta += \Delta \theta$
    
\ENDFOR

\STATE return $\{V\}$
\end{algorithmic} 
\end{algorithm}

%\nisarcomm{...once again, you need to provide an algorithm here to summarize the recipe you seem to be verbally implying above, i.e. that there is  a process by which one samples vertices, and angles in some particular way/order, but it is not precisely clear what that order is, or how to initialize, or when to terminate, or what the tuning knobs are, etc. ..again, someone has to be able to implement this...}
% The full PSEUD algorithm is further specified in \ref{alg:PSEUD}. 
Using PSEUD, sketches can be drawn from the distribution of sketches carrying the same parameterization, allowing high fidelity testing of each parameters effect on POMDP performance. These sketches, represented by their vertices can then be directly converted into softmax observation models using the techniques of \cite{sweet2016structured}, as described in 5.7.1. For example, both of the sketches shown in Figure \ref{fig:pseud_Draws} are drawn from a single parameterizied distribution, and yield similarly structured softmax models.

\begin{figure}[h!]
    \centering	
    \begin{subfigure}{0.45\textwidth}
        \includegraphics[width=1\textwidth]{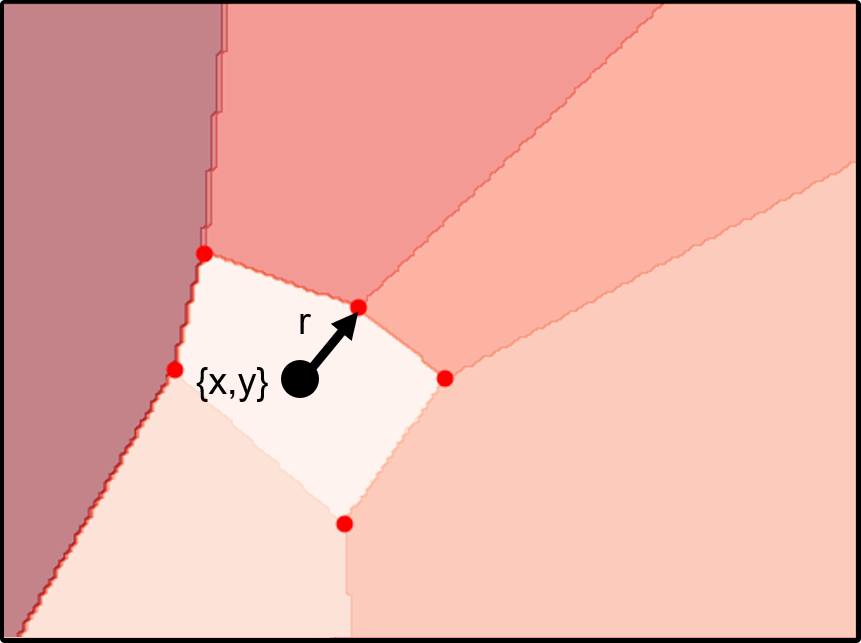}
    \end{subfigure}
    ~    
    \begin{subfigure}{0.45\textwidth}
        \includegraphics[width=1\textwidth]{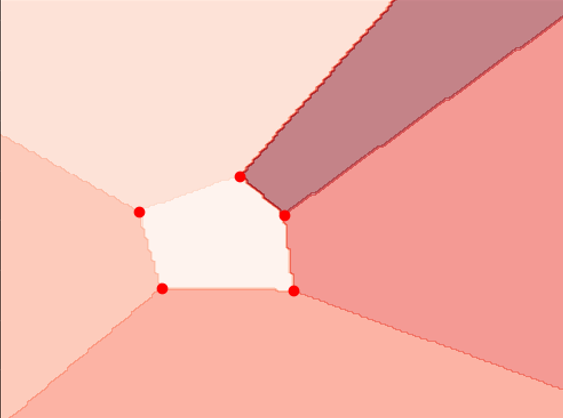}
    \end{subfigure}
    \caption{Two draws from the PSEUD Algorithm for a given centroid \{x,y\} and radius $(r)$}
    \label{fig:pseud_Draws}
    \vspace{-0.15in}
\end{figure}

\subsection{Monte Carlo Auto-labeling}
%Discussion of Need for Auto-labeling
%\nisarcomm{note: no dash in `Monte Carlo'...}
Once a softmax observation model has been generated, whether by a real human or through a simulator such as PSEUD, the individual softmax classes can be mapped onto semantic labels for further human interaction. In the Cops and Robots experiment of \cite{burks2021collaborative}, this mapping was largely defined by hand offline to be 1-to-1, with a particular class label index always corresponding to `South' for instance. This was enabled by assuming that the 2D spatial extent of all known semantic reference objects could be represented by simple Cartesian-aligned rectangles, so that softmax parameters for semantic classes describing 4 canonical  bearings relative to the reference object needed to be specified. The use of free-form ad hoc sketches leaves little room for such restrictions. For instance, in either of the sketches in Figure \ref{fig:pseud_Draws}, it is unclear which of the classes would receive the exclusive use of the label `North', and indeed it seems unwieldy to attempt such a hard classification.  This suggests that a soft classification approach could be used, disassociating the semantic labels from tight correspondence with individual classes.

%Formal definitions and math
%\nisarcomm{you need to be more careful/precise here from this paragraph on: the notation for this subsection is disjointed and disconnected from what came earlier -- you start by defining new random variables `class' and `label' without saying what they actually mean, but then you use $c$ and $l$ as shorthands later without saying this; and then later refer to using $p(c|l)$ `within the Bayesian belief update to find $p(s|l)$' and $p(l|c)$ is used to generate semantic labels from belief states during planning phase through $p(l|s)$, even though the POMDP's updates are based on observations $o_h$, not $l$ --- point is: you need to reconcile the notations here with what you ultimately use for the POMDP math setup and planning description...}

To start this process, a new set of conditional probabilities are defined as the probability that a state drawn from softmax class $(c)$ would be associated with the relational label $(l)$, $p(label=l | class = c)$, and the probability that a given human observation $o_{h}$ arising from a query action $a_{q}$ corresponding to semantic label $l$ was referring to the current state being associated with softmax class $c$, $p(class=c|a_{q} = l, o_{h} = Yes)$, or more succinctly $p(class=c|label=l)$. That is, given that the human indicated the state was associated with relational label $(l)$, with what probability the true state would have been drawn from softmax class $(c)$ The generative process used to build the POMCP planning tree will rely on $p(label=l | class=c)$, $p(l|c)$ for short, while updating the target belief distribution requires $p(class=c|label=l)$, $p(c|l)$.
Both conditional distributions can be derived from the joint probability distribution $p(c,l)$. 
In order to find this distribution, first a canonical semantic bearing model $L$ with overlapping 90 degree increments is assumed. Each semantic label, corresponding to the 8-point set of cardinal directions, covers an angular distance of 90 degrees, and overlaps by 45 degrees with the labels on either side. For instance, a point at $\frac{\pi}{4}$ radians or 45 degrees counterclockwise above the horizontal in this canonical model can be accurately labeled `North', `NorthEast', or `East', while a point at 60 degrees counterclockwise above the horizontal can be labeled only `North' or `NorthEast'. Such a model can be represented as an overlapping piece-wise function on the angle $\theta$ made by state $(s)$ with the horizontal, generating labels $(l)$,

\begin{align}
    L(s) = 
    \begin{cases} 
      NorthEast & 0\leq \theta \leq 90 \\
      North & 45\leq \theta \leq 135 \\
      NorthWest & 90\leq \theta \leq 180 \\
      West & 135\leq \theta \leq 225 \\
      ...
   \end{cases}
\end{align}
Note, the overlapping nature of this function allows for the return of a set of labels, rather than a single label. This further suggests the possibility of a softmax representation, which will be explored in future work. Here the probabilistic representation $p(l \in L(s) | s)$ is used to describe the current deterministic function to preserve generality. 

In order to find the joint probability $p(c,l)$, it is necessary to calculate the integral of the product of the class and label probability over the state space. 

\begin{align}
    p(c,l) = \int_{s \in S} p(c|s)p(l \in L(s)|s) ds
\end{align}

While the label term $p(l\in L(s) | s)$ can only take values 0 or 1, as it describes a deterministic piece-wise function, the integral over the softmax function $p(c|s)$ is analytically intractable \cite{ahmed2013bayesian}. Therefore, a Monte Carlo approach is used to approximate the integral, selecting $J$ states $s \in \mathcal{S}$ to carry out the summation:

\begin{align}
    p(c,l) = \frac{1}{J} \sum_{j=1}^{J} p(c|s_{j}) p(l \in L(s_{j})|s_{j})
\end{align}

From this joint distribution, both the conditional probabilities $p(c|l)$ and $p(l|c)$ can be easily obtained. The former is used within the Bayesian belief update to find $p(s|l)$,

\begin{align}
    p(s|l) = \sum_{c}p(s|c)p(c|l)
\end{align}

while the later is used to generate semantic labels from belief states during the planning phase through $p(l|s)$,

\begin{align}
    p(l|s) = \sum_{c}p(l|c)p(c|s)
\end{align}
Again, in this instance $p(c|l)$ corresponds to $p(class=c|a_{q} = l, o_{h} = Yes)$, such it serves as a probabilistic mapping from human information to a set of mathematical objects after a robotic query. 

While this approximation approaches the true joint distribution with infinite samples, it is necessary in practice to choose a finite number of points. While these would typically be randomly scattered throughout the state space to avoid sampling bias, the number of points required to achieve an accurate approximation could be rather high. To limit computational expense, while preserving the approximation's accuracy, this work leverages the determinism and radial symmetry of the piece-wise canonical bearing model $L$ by using a set of points uniformly distributed on $\theta$ at a constant radius. This method is illustrated in Figure \ref{fig:autolabeling}, where the softmax model on the left is evaluated using the ring of Monte Carlo points on the right.

%Figure
\begin{figure}[h]
    \centering	
    \begin{subfigure}{0.45\textwidth}
        \includegraphics[width=1\textwidth]{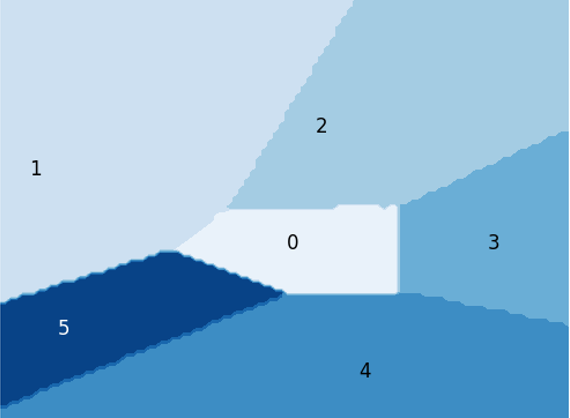}
    \end{subfigure}
    ~    
    \begin{subfigure}{0.45\textwidth}
        \includegraphics[width=1\textwidth]{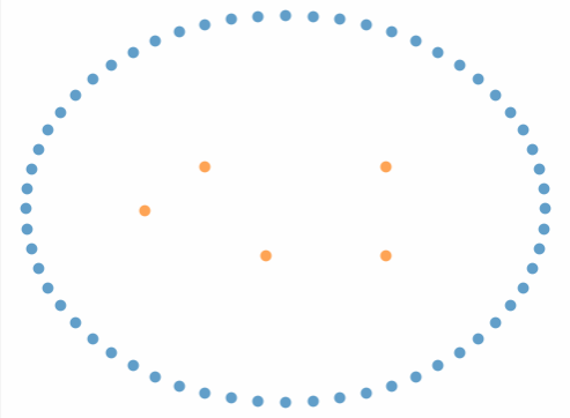}
    \end{subfigure}
    \caption{An irregular softmax model with numbered class labels (left)\\ The Monte Carlo approximation points used to approximate semantic class labels (right)}
    \label{fig:autolabeling}
    \vspace{-0.15in}
\end{figure}

This approximation yields the conditional probability distributions shown in Figure \ref{fig:autoConditionals}. These distributions, substantially similar to those found using a dense random sampling method with 10000 points, were found using only a sampled ring of 360 points. Furthermore, they correspond to intuition regarding the semantic labels. From model in Figure \ref{fig:autolabeling}, $p(class|label)$ in Figure \ref{fig:autoConditionals} indicates that an observation `South' of the object in question could only reasonably be associated with class 4, while $p(label|class)$ indicates that states sampled from class 4 would likely be labeled either `SouthWest', `South', or `SouthEast'. 
%\nisarcomm{are these values close to the ones from using the denser sampling method?}

\begin{figure}[h!]
    \centering	
    \begin{subfigure}{0.45\textwidth}
        \includegraphics[width=1\textwidth]{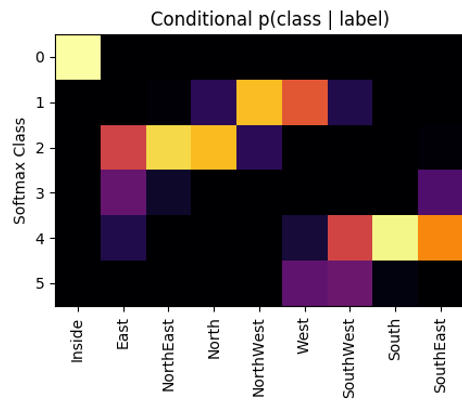}
    \end{subfigure}
    ~    
    \begin{subfigure}{0.45\textwidth}
        \includegraphics[width=1\textwidth]{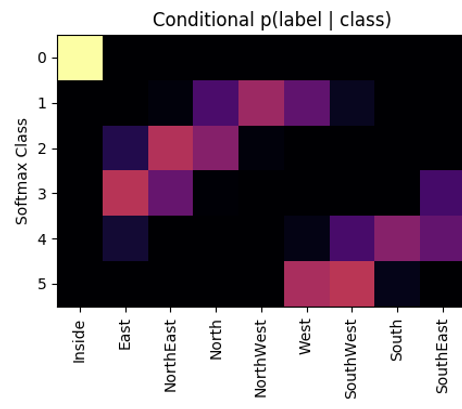}
    \end{subfigure}
    \caption{Conditional probability tables derived from Monte Carlo Auto-labeling}
    \label{fig:autoConditionals}
    \vspace{-0.15in}
\end{figure}

\subsection{Composite Range Models}
%Discussion of Need for Composite Near
While the Monte Carlo Auto-labeling technique described in the previous section establishes a probabilistic correspondence between softmax classes and the type of semantic labels a human would use, the interior class based method of building softmax models used in \cite{burks2019optimal,burks2018closed,burks2019collaborative} is limited in its ability to express range information. The target can be described as ``Inside" the sketch if it is literally within the bounds of the sketched convex polygon, or as ``Not Inside", in which case it can be anywhere else in the state space. In many applications, including the motivating problem for this work, it is desirable to express when the target is in the general vicinity of the sketch, when it is ``Near" or ``Near NorthEast" to a particular landmark. Previous work \cite{ahmed2013bayesian} constructed such range-bearing softmax models using hand crafted classes for specific range-bearing combinations (``Near Northeast"), and used an multimodal softmax (MMS) model summing together a set of classes to express range only measurements (``Near"). 

Here an alternative method is proposed for constructing range labels which is more applicable to ad hoc sketch-based softmax models. Here, the range softmax model is constructed based on the structure of the sketch before being combined with the sketched bearing model in a product softmax model \cite{sweet2016structured}. Specifically, this section and the following text make use of a single label ``Near" range model, rather than the multiple option range models of previous work.

%Formal definitions and math
The ``Near'' class is first assumed to hold an identical, yet inflated, shape to the original interior softmax class, which has conditional probability $p(Inside|s)$. That is to say, the vertices of the near model are an affine transform of the original vertices such that the area they encompass is a scalar multiple $h$ of the previous area. The interior class of these inflated points can be applied as a product softmax model as shown in \ref{fig:nearComposite}, under the assumption that range and bearing are independent, such that

\begin{align}
\label{eq:indRangeBear}
    p(Near,Bearing|s) = p(Near|s)p(Bearing|s)
\end{align}

Thus, a point can be evaluated against both models separately to determine the probability it was drawn from the composite joint range-bearing class label. This work only considers the use of the ``Near" range observation, with observations outside the range models interior class carrying no explicit range information. In such a framework, the negative observation ``Not Near" serves as a proxy for the implicit observation ``Far". In principle, rather than being restricted to binary range information, additional affine transforms of larger size can be applied to indicate any number of semantic ranges. However, such models would necessarily overlap and fully contain the smaller ``Near" interior class, such that for some hypothetical ``Near/Far" range model it must be assumed that any observation ``Far" is actually the compound observation ``Far and Not Near":

\begin{align}
    p(Far,~Near|s) = p(Far|s)(1-p(Near|s))
\end{align}

In this way, Eq. \ref{eq:indRangeBear} can be generalized, with the assumption of range-bearing independence intact, to: 
\begin{align}
    p(Range,Bearing|s) = p(Range|s)p(Bearing|s)
\end{align}

A cleaner approach to be explored in future work would be the use of softmax models specified directly in range space, such that ``Near" and ``Far" could correspond to 2 different classes within the same function rather than 2 separate functions. However, this approach would neglect the shape information from the sketch preserved in the affine transform method, a trade-off to be further explored. The example problems in the following sections are restricted to the ``Near" only range models. 

%However, it is possible that as distance increases, the affine transforms key feature of preserving the original sketch's shape may become less advantageous, while softmax functions constructed direc
% \lukecomm{Include additional equation generalizing to additional ranges while removing near info} 
% \nisarcomm{is this true just for the ``Near'' class, or all possible range classes? If only for ``Near'' class and you are deliberately ignoring other classes, you should make this clearer earlier on...
% If for multiple range classes, then should replace ``Near'' in above desc with a Range variable, which takes on a discrete set of semantic range values (how does the upper semantic range limit get set?)...example above is for Fig 5.13 but seems like the math is more general than just for the one range class..}

%Figure
\begin{figure}[h]
\centering	
    \includegraphics[width=.45\textwidth]{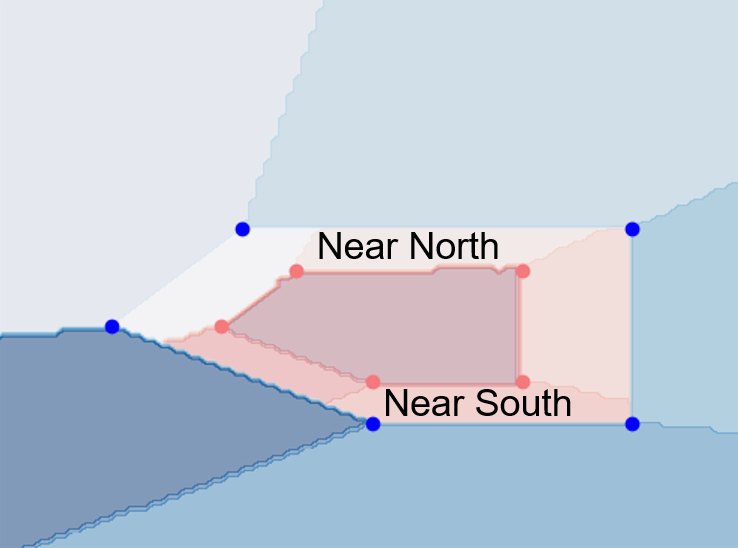}
	\caption{Composite Range and Bearing Softmax Model}
    \label{fig:nearComposite}
\end{figure}
